# Supplementary material for: SCION: Scene Composition with Instanced Neural Primitives
Source: arXiv:2610.02322 source file (2026-10-05)
Supplement: Supplementary file 1 [file supp_labels.tex]

\makeatletter
\newlabel{sec:appendix-architecture}{{S1}{1}{}{}{}}
\newlabel{sec:appendix-initialization}{{S1.1}{1}{}{}{}}
\newlabel{eq:dino-init}{{S1.1}{1}{}{}{}}
\newlabel{eq:codebook-init}{{S1.1}{1}{}{}{}}
\newlabel{sec:appendix-reg}{{S1.2}{1}{}{}{}}
\newlabel{eq:reg-scale}{{S1.2}{1}{}{}{}}
\newlabel{eq:reg-opacity}{{S1.2}{1}{}{}{}}
\newlabel{sec:appendix-discriminator}{{S1.3}{2}{}{}{}}
\newlabel{eq:adv-d}{{S1}{2}{}{}{}}
\newlabel{eq:adv-g}{{S2}{2}{}{}{}}
\newlabel{sec:appendix-mh-splat}{{S1.4}{2}{}{}{}}
\newlabel{eq:mh-importance}{{S3}{2}{}{}{}}
\newlabel{eq:mh-accept}{{S4}{2}{}{}{}}
\newlabel{eq:mass-relocation}{{S5}{2}{}{}{}}
\newlabel{sec:appendix-algorithms}{{S1.5}{2}{}{}{}}
\newlabel{alg:splat-mh}{{S1}{3}{}{}{}}
\newlabel{sec:appendix-edit-animation}{{S1.6}{3}{}{}{}}
\newlabel{alg:inst-default}{{S2}{4}{}{}{}}
\newlabel{sec:appendix-hyperparams}{{S1.7}{4}{}{}{}}
\newlabel{sec:appendix-compute}{{S1.8}{5}{}{}{}}
\newlabel{sec:appendix-results}{{S2}{5}{}{}{}}
\newlabel{sec:appendix-full-results}{{S2.1}{5}{}{}{}}
\newlabel{tab:main_results}{{S1}{5}{}{}{}}
\newlabel{sec:appendix-ablations}{{S2.2}{5}{}{}{}}
\newlabel{tab:capacity_ablation}{{S2}{6}{}{}{}}
\makeatother
